# Supplementary material for: The Early Universe as a Probe of New Physics
Source: arXiv:0812.4494 source file (2008-12-24)
Supplement: Supplementary file 1 [file appendix1.tex]

\chapter*{A Short History of the Universe}

\begin{itemize}
\item {\bf The Big Bang} - The universe is created, quantum gravity dominates the physics
\item {\bf $10^{-36} - 10^{-34} s$} - Grand Unified Theories are broken, and defects are created
\item {\bf $10^{-30} $s } - Inflation and reheating of the universe ends
\item {\bf 
Thermal and Non-Thermal Kaluza-Klein Modes are Created
}

\item {\bf $10^{-12} $s } - Electroweak symmetry is broken
\item {\bf $10^{-6} - 10^{-5}$ s} - WIMPs freeze out
\item {\bf 
Minimal Dark Matter Models Freeze Out
 }
\item {\bf $10^{-5} $s} - Quarks form into hadrons
\item {\bf 3 minutes} - Big Bang nucleosynthesis has formed most of the light elements
\item {\bf 
Quasistable CHAMPs Form Bound States and Catalyze Nucleosynthesis
}
\item {\bf 
Kaluza-Klein Modes Destroy \lisx\ Nuclei
}
\item {\bf 200,000 years} - The cosmic microwave background forms
\item {\bf 1,000,000 years} - Early galaxies begin forming
\item {\bf 
Cosmic Kaluza-Klein Modes are Trapped in the Galaxy
}
\item {\bf 10,000,000,000 years} - The Earth and Solar System form
\item {\bf 14,700,000,000 years} - Astrophysics experiments can probe the early Universe

\item {\bf 
Dedicated Detectors Search for Dark Matter
}

\item {\bf 
The Large Hadron Collider Starts Searching for Dark Matter and Extra Dimensions
}

\end{itemize}
